# Supplementary material for: Towards Learning High-Precision Least Squares Algorithms with Sequence Models
Source: arXiv:2503.12295 source file (2025-03-15)
Supplement: Supplementary file 1 [file linear_attn_square.tex]

\subsubsection{Linear attention can't implement element-wise squaring.}\label{app:attn_square}
In this section, we consider the following parameterization of \textit{linear attention}:
\begin{equation}
    \text{LinearAttn}(\bm{u}) = (\bm{u} \bm{W}_{\bm{Q}}) (\bm{u} \bm{W}_{\bm{K}})^T (\bm{u} \bm{W}_{\bm{V}} + \bm{B}),
\end{equation}
where $\bm{u} \in \mathbb{R}^{\seqLen \times \hiddenDim}$, $\bm{W}_{\bm{Q}}, \bm{W}_{\bm{K}}, \bm{W}_{\bm{V}} \in \mathbb{R}^{\hiddenDim \times \hiddenDim}$ and $\bm{B} \in \mathbb{R}^{\seqLen \times \hiddenDim}$.
\theorem{
    One-layer linear attention cannot exactly represent the entry-wise squaring function $\textsc{Square} : \mathbb{R}^{\seqLen \times \hiddenDim} \to \mathbb{R}^{\seqLen \times \hiddenDim}$ s.t.
    $$\textsc{Square}(\bm{u})_{ij} = \bm{u}_{ij}^2$$
    for all $\bm{u} \in \mathbb{R}^{\seqLen \times \hiddenDim}$.
}\label{thm:attn_square_app}
\proof{
    We proceed by contradiction. Let's assume there exists $\bm{W}_{\bm{Q}}, \bm{W}_{\bm{K}}, \bm{W}_{\bm{V}} \in \mathbb{R}^{\hiddenDim \times \hiddenDim}$ and $\bm{B} \in \mathbb{R}^{\seqLen \times \hiddenDim}$ such that $\forall \bm{u} \in \mathbb{R}^{\seqLen \times \hiddenDim}$,
    \begin{equation}
        (\bm{u} \bm{W}_{Q}) (\bm{u} \bm{W}_{K})^T (\bm{u} \bm{W}_{V} + \bm{B}) = \textsc{Square}(\bm{u}).
    \end{equation}
    Consider the set of inputs $\bm{u} \in \mathbb{R}^{\seqLen \times \hiddenDim}$ with two non-zero entries, defined as
    \begin{equation}
        \bm{u}_{ij} =
        \begin{cases}
            \bm{u}_{ij} & (i, j) \in \{(a, c), (b, d)\} \\
            0 & \text{else}
        \end{cases}
    \end{equation}
    for an arbitrary choice of $a, b \in [\seqLen]$, $c, d \in [\hiddenDim]$. Then:
    \begin{equation}
        \bm{Q} := \bm{u} \bm{W}_{\bm{Q}} =
        \begin{pmatrix}
            \bm{0}^\seqLen \\
            \hline \\
            \vdots \\
            \hline \\
            \bm{0}^\seqLen \\
            \hline \\
            \bm{u}_{ac} \bm{W}_{\bm{Q}}[c, :] \\
            \hline \\
            \bm{0}^\seqLen \\
            \hline \\
            \vdots \\
            \hline \\
            \bm{0}^\seqLen \\
            \hline \\
            \bm{u}_{bd} \bm{W}_{\bm{Q}}[d, :] \\
            \hline \\
            \bm{0}^\seqLen \\
            \hline \\
            \vdots \\
            \hline \\
            \bm{0}^\seqLen
        \end{pmatrix}
    \end{equation}
    where $\bm{Q}$'s rows are all $\bm{0}$ except for the $a$-th and $b$-th, which are $\bm{u}_{ac} \bm{W}_{\bm{Q}}[c, :]$ and $\bm{u}_{bd} \bm{W}_{\bm{Q}}[d, :]$ respectively.

    Similarly:
    \begin{equation}
        \bm{K} := \bm{u} \bm{W}_{\bm{K}} =
        \begin{pmatrix}
            \bm{0}^\seqLen \\
            \hline \\
            \vdots \\
            \hline \\
            \bm{0}^\seqLen \\
            \hline \\
            \bm{u}_{ac} \bm{W}_{\bm{K}}[c, :] \\
            \hline \\
            \bm{0}^\seqLen \\
            \hline \\
            \vdots \\
            \hline \\
            \bm{0}^\seqLen \\
            \hline \\
            \bm{u}_{bd} \bm{W}_{\bm{K}}[d, :] \\
            \hline \\
            \bm{0}^\seqLen \\
            \hline \\
            \vdots \\
            \hline \\
            \bm{0}^\seqLen
        \end{pmatrix}
    \end{equation}
    and
    \begin{equation}
        \bm{V} := \bm{u} \bm{W}_{\bm{V}} =
        \begin{pmatrix}
            \bm{0}^\seqLen \\
            \hline \\
            \vdots \\
            \hline \\
            \bm{0}^\seqLen \\
            \hline \\
            \bm{u}_{ac} \bm{W}_{\bm{V}}[c, :] \\
            \hline \\
            \bm{0}^\seqLen \\
            \hline \\
            \vdots \\
            \hline \\
            \bm{0}^\seqLen \\
            \hline \\
            \bm{u}_{bd} \bm{W}_{\bm{V}}[d, :] \\
            \hline \\
            \bm{0}^\seqLen \\
            \hline \\
            \vdots \\
            \hline \\
            \bm{0}^\seqLen
        \end{pmatrix}
    \end{equation}

    Then the attention matrix, $\bm{A} = \bm{Q} \bm{K}^T$, satisfies
    \begin{equation}
         \bm{A}_{ij} =
        \begin{cases}
            \bm{u}_{ac}^2 (\bm{W}_{\bm{Q}} \bm{W}_{\bm{K}}^T)_{cc} & (i, j) = (a, a) \\
            \bm{u}_{ac} \bm{u}_{bd} (\bm{W}_{\bm{Q}} \bm{W}_{\bm{K}}^T)_{cd} & (i, j) = (a, b) \\
            \bm{u}_{ac} \bm{u}_{bd} (\bm{W}_{\bm{Q}} \bm{W}_{\bm{K}}^T)_{dc} & (i, j) = (b, a) \\
            \bm{u}_{bd}^2 (\bm{W}_{\bm{Q}} \bm{W}_{\bm{K}}^T)_{dd} & (i, j) = (b, b) \\
            0 & \text{else}
        \end{cases}.
    \end{equation}

    Now let's consider the output of linear attention:
    \begin{equation}
        \bm{O} = (\bm{Q}\bm{K}^T)(\bm{V} + \bm{B})
    \end{equation}
    such that $\bm{O} = \textsc{Square}(\bm{u})$.

    \paragraph{Case 1: $\bm{B} = \bm{0}$.}
    We have
    \begin{equation}
        \bm{O}[a, :] = \bm{u}_{ac}^3 (\bm{W}_{\bm{Q}} \bm{W}_{\bm{K}}^T)_{cc} \bm{W}_{\bm{V}}[c, :] + \bm{u}_{ac} \bm{u}_{bd}^2 (\bm{W}_{\bm{Q}} \bm{W}_{\bm{K}}^T)_{cd} \bm{W}_{\bm{V}}[d, :]
    \end{equation}
    and
    \begin{equation}
        \bm{O}[b, :] = \bm{u}_{ac}^2 \bm{u}_{bd} (\bm{W}_{\bm{Q}} \bm{W}_{\bm{K}}^T)_{dc} \bm{W}_{\bm{V}}[c, :] + \bm{u}_{bd}^3 (\bm{W}_{\bm{Q}} \bm{W}_{\bm{K}}^T)_{dd} \bm{W}_{\bm{V}}[d, :]
    \end{equation}
    Note that each term of the output is a cubic polynomial of the inputs $\bm{u}_{ac}$ and $\bm{u}_{bd}$, whereas our target $\textsc{Square}(\bm{u})$ consists of quadratic polynomials, so these cannot be exactly equivalent.

    \paragraph{Case 2: $\bm{B} \neq \bm{0}$.}
    In this case,
    \begin{equation}\label{eqn:attn_square_app_case2_eq1}
        \bm{O}[a, :] = \bm{u}_{ac}^3 (\bm{W}_{\bm{Q}} \bm{W}_{\bm{K}}^T)_{cc} \bm{W}_{\bm{V}}[c, :] + \bm{u}_{ac}^2 (\bm{W}_{\bm{Q}} \bm{W}_{\bm{K}}^T)_{cc} \bm{B}[a, :] + \bm{u}_{ac} \bm{u}_{bd}^2 (\bm{W}_{\bm{Q}} \bm{W}_{\bm{K}}^T)_{cd} \bm{W}_{\bm{V}}[d, :] + \bm{u}_{ac} \bm{u}_{bd} (\bm{W}_{\bm{Q}} \bm{W}_{\bm{K}}^T)_{cd} \bm{B}[b, :]
    \end{equation}
    and
    \begin{equation}\label{eqn:attn_square_app_case2_eq2}
        \bm{O}[b, :] = \bm{u}_{ac}^2 \bm{u}_{bd} (\bm{W}_{\bm{Q}} \bm{W}_{\bm{K}}^T)_{dc} \bm{W}_{\bm{V}}[c, :] + \bm{u}_{ac} \bm{u}_{bd} (\bm{W}_{\bm{Q}} \bm{W}_{\bm{K}}^T)_{dc} \bm{B}[a, :] + \bm{u}_{bd}^3 (\bm{W}_{\bm{Q}} \bm{W}_{\bm{K}}^T)_{dd} \bm{W}_{\bm{V}}[d, :] + \bm{u}_{bd}^2 (\bm{W}_{\bm{Q}} \bm{W}_{\bm{K}})_{dd} \bm{B}[b, :]
    \end{equation}
    In order for $\bm{O} = \textsc{Square}(\bm{u})$, we need \begin{equation}\label{eqn:attn_square_app_case2_eq3}
        \bm{O}[a, :] = \bm{u}_{ac}^2 \bm{e}_c^\hiddenDim, \quad \bm{O}[b, :] = \bm{u}_{bd}^2 \bm{e}_d^\hiddenDim
    \end{equation}
    Then, setting the quadratic terms of Equation~\ref{eqn:attn_square_app_case2_eq3} and Equations~\ref{eqn:attn_square_app_case2_eq1}, \ref{eqn:attn_square_app_case2_eq2} equal, we must have
    \begin{equation}
        (\bm{W}_{\bm{Q}} \bm{W}_{\bm{K}}^T)_{cc} = (\bm{W}_{\bm{Q}} \bm{W}_{\bm{K}}^T)_{dd} = 1
    \end{equation}
    and
    \begin{equation}
        \bm{B}[a, :] = \bm{e}_a^\hiddenDim, \quad \bm{B}[b, :] = \bm{e}_b^\hiddenDim
    \end{equation}
    The cubic terms in Equations~\ref{eqn:attn_square_app_case2_eq1}, \ref{eqn:attn_square_app_case2_eq2} must also vanish, which implies
    \begin{equation}
        \bm{W}_{\bm{V}}[c, :] = \bm{W}_{\bm{V}}[d, :] = \bm{0}^\hiddenDim.
    \end{equation}
    The $\bm{u}_{ac} \bm{u}_{bd}$ terms must also vanish, which implies
    \begin{equation}
        (\bm{W}_{\bm{Q}} \bm{W}_{\bm{K}}^T)_{cd} = (\bm{W}_{\bm{Q}} \bm{W}_{\bm{K}}^T)_{dc} = 0.
    \end{equation}

    Finally, note that the above must hold for all choices of $a, b \in [\seqLen]$ and $c, d \in [\hiddenDim]$. This implies that we have:
    \begin{equation}
        \bm{V} = \bm{0}^{\hiddenDim \times \hiddenDim}, \quad, \bm{B} = \bm{I}^{\hiddenDim \times \hiddenDim}, \quad \bm{W}_{\bm{Q}}\bm{W}_{\bm{K}}^T = \bm{I}^{\hiddenDim \times \hiddenDim}
    \end{equation}

    In other words, the set of constraints from our arguments above fully specify the weights of linear attention. However, we can verify that these weights fail to express $\textsc{Square}$ by evaluating the linear attention:
    \begin{equation}
        (\bm{W}_{\bm{Q}} \bm{W}_{\bm{K}}^T)(\bm{V} + \bm{B}) = (\bm{u}\bm{W}_{\bm{Q}} \bm{W}_{\bm{K}}^T \bm{u}^T)(\bm{u}\bm{V} + \bm{B}) = (\bm{u}\bm{u}^T)(\bm{0}^{\hiddenDim \times \hiddenDim} + \bm{I}^{\hiddenDim \times \hiddenDim}) = \bm{u}\bm{u}^T
    \end{equation}
    However, it is easy to check that $ \bm{u}\bm{u}^T \neq \textsc{Square}(\bm{u})$, which completes the proof by contradiction.
}

\newpage
